# Supplementary material for: Perfect separation of intraband and interband excitations in PdCoO$_2$
Source: arXiv:1811.01026 source file (2019-05-06)
Supplement: Supplementary file 1 [file supplemental.pdf]

# Supplementary Material for: Perfect separation of intraband and interband excitations in $PdCoO_2$

C. C. Homes,[1,*] S. Khim,[2] and A. P. Mackenzie[2,3,†]

[1]*Condensed Matter Physics and Materials Science Division, Brookhaven National Laboratory, Upton, New York 11973, USA*
[2]*Max Planck Institute for Chemical Physics of Solids, Nöthnitzer Strasse 40, 01187 Dresden, Germany*
[3]*Scottish Universities Physics Alliance, School of Physics & Astronomy, Universtiy of St. Andrews, North Haugh, St. Andrews KY16 9SS, United Kingdom*

(Dated: April 23, 2019)

## ELECTRONIC STRUCTURE CALCULATIONS

The delafossite $PdCoO_2$ crystalizes in the trigonal $R\bar{3}m$ (166) space group, consisting of Pd triangular layers and $CoO_2$ triangular slabs [1]. The electronic properties have been calculated using density functional theory (DFT) with the generalized gradient approximation (GGA) using the full-potential linearized augmented plane-wave (FP-LAPW) method [2] with local-orbital extensions [3] in the WIEN2k implementation [4]. An examination of different Monkhorst-Pack $k$-point meshes indicated that a $5 \times 5 \times 5$ $k$-point mesh with $R_{mt}k_{max} = 8$ was sufficient for good energy convergence. Beginning with the experimental unit cell [1] $a = 2.83$ and $c = 17.743$ Å, with the atomic positions of Pd, Co and O at $(0, 0, 0)$, $(0, 0, \frac{1}{2})$, and $(0, 0, 0.1064)$, respectively, the total energy was minimized by adjusting $a$ and $c$ axes; the atomic fractional coordinate for the oxygen atom was then relaxed with respect to the total force, typically resulting in residual forces of less than 0.1 mRy/a.u. per atom. This procedure was repeated until no further improvement was obtained, yielding $a = 2.876$ and $c = 17.972$ Å; the position of the oxygen atom has shifted slightly to $(0, 0, 0.1131)$. For both of these procedures spin-orbit coupling is ignored.

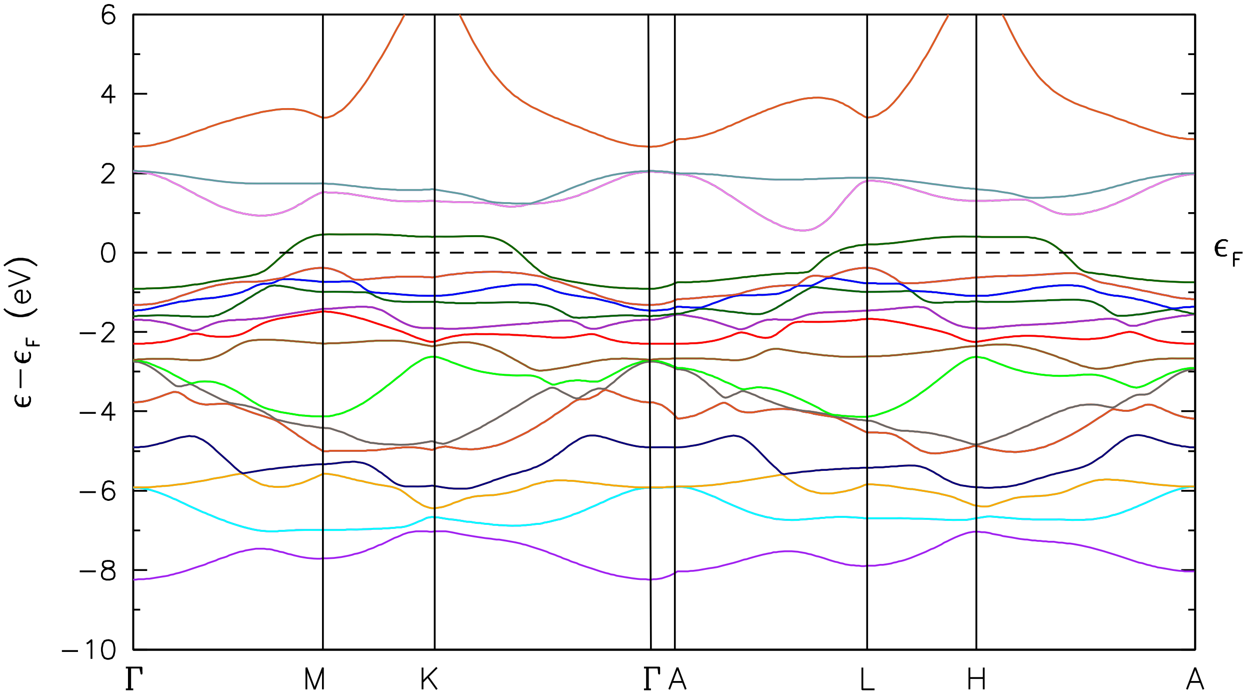


Figure S1. The calculated GGA electronic band structure of $PdCoO_2$ including the effects of spin-orbit coupling shown for several different paths between high-symmetry points for a trigonal Brillouin zone (generated using 400 $k$ points).

The electronic band structure has been calculated with GGA and spin-orbit coupling for several different paths between high-symmetry points in the trigonal unit cell, shown in Fig. S1. This calculation accurately reproduces the

Typeset by REVTEX

results of several other calculations [5–8]. As Fig. S1 indicates, there is only a single band crossing the Fermi surface, which has been attributed to the Pd $4d_{3z^2-r^2}$–Pd $5s$ hybridized state [6]. While the paths along the high-symmetry directions are useful, the contribution of the bands to the transport is better understood from the nature of the Fermi surface.

## FERMI SURFACE

The Fermi surface has been calculated using GGA and a large number of $k$-points (10 000 $k$ points, resulting in a $21 \times 21 \times 21$ mesh). The resulting Fermi surface is shown in Fig. S2 and consists of a large warped hexagonal sheet, in agreement with previous calculations [6, 8] and experimental results [9, 10].

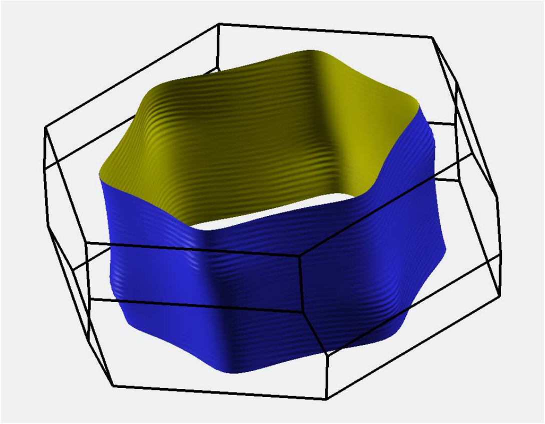

Figure S2. The Fermi surface of $PdCoO_2$ in the first Brillouin zone.

## DIELECTRIC TENSOR AND OPTICAL CONDUCTIVITY

The real part of the optical conductivity has been determined [11] from the imaginary part of the dielectric function for $\sigma_{x,x} = 2\pi\omega\,\Im\,\epsilon_{x,x}/Z_0$ ($a$ axis), and $\sigma_{z,z} = 2\pi\omega\,\Im\,\epsilon_{z,z}/Z_0$ ($c$ axis), shown in Fig. S3, using a fine $k$ point mesh (10 000 $k$ points, yielding a $21 \times 21 \times 21$ mesh); $Z_0 \approx 377\,\Omega$ is the impedance of free space, resulting the units for the conductivity of $\Omega^{-1}\mathrm{cm}^{-1}$. Initially, the free-carrier contribution is not calculated, so that the imaginary part of the dielectric function is the sum of the contributions to the dielectric tensor over all the allowed interband transitions; only direct ($\mathbf{q} = 0$) transitions are considered from occupied to unoccupied states. The onset of absorption is observed to occur at $\simeq 4000$ cm$^{-1}$, with a strong peak at $\simeq 7000$ cm$^{-1}$ along the $a$-axis direction (somewhat higher along the $c$ axis), very close to where the onset of absorption is observed in the experimental data. The intraband contributions have been calculated for the $a$ and $c$ axes with values of $\omega_{p,a} \simeq 31\,500$ cm$^{-1}$ and $\omega_{p,c} \simeq 3660$ cm$^{-1}$, respectively. This indicates a large anisotropy in the effective mass of $\omega_{p,a}^2/\omega_{p,c}^2 = m_c^*/m_a^* \simeq 74$.

## LATTICE DYNAMICS

The lattice vibrations have been determined using the direct method, also known as the frozen-phonon technique. To determine the phonons at the zone center, a $1 \times 1 \times 1$ supercell is sufficient. To obtain a complete set of Hellmann-Feynman forces, a total of 9 independent displacements are required; because there are always some residual forces at the atomic sites we have considered symmetric displacements, which doubles this number, resulting in a total of 18 atomic displacements. In this case, displacement amplitudes of 0.03 Å were used; typical values for the displacements range from 0.02 to 0.06 Å. The atomic displacements lower the symmetry of the unit cell resulting in a $10 \times 10 \times 1$ $k$-point mesh. The calculations have converged when the successive changes for the forces on each atom are less than 0.01 mRy/a.u. The residual forces are collected for each set of symmetric displacements and a list of the Hellmann-Feynman forces are generated. Using the program PHONON [12] the cumulative force constants deconvoluted from the Hellmann-Feynman forces are introduced into the dynamical matrix, which is then diagonalized in order to obtain

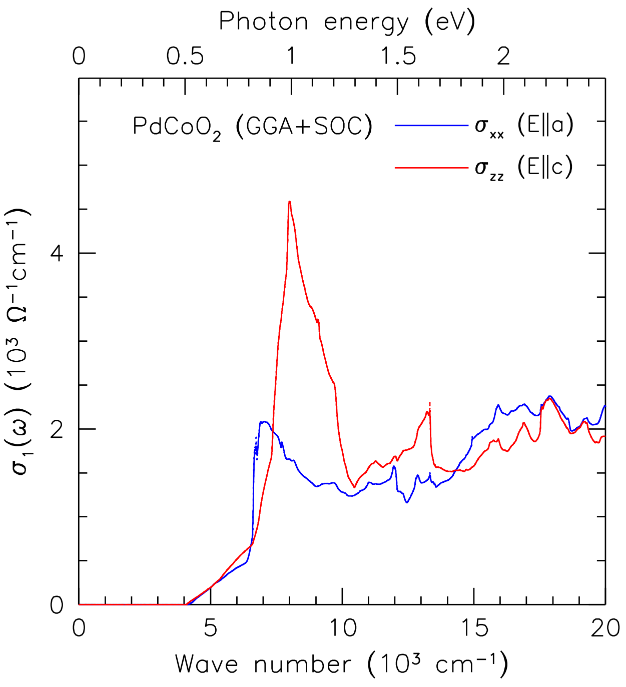


Figure S3. The calculated result for the real part of the optical conductivity for $PdCoO_2$ along the $x$ ($a$) and $z$ ($c$) directions.

the phonon frequencies. The atomic intensities are further calculated to describe the character of the vibration; in this case the intensity refers to the square of the vibrational amplitude of each atom for a given mode. The results of the calculation are comparison with experimental results are summarized in Table I.

Table I. Experimental and calculated frequencies and atomic intensities for $PdCoO_2$.

| | | | | | | Atomic Intensity | |
|---|---|---|---|---|---|---|---|
| Mode | $\omega_{exp}$ (cm$^{-1}$) | $\omega_{calc}$ (cm$^{-1}$) | Type | Activity | Pd | Co | O |
| $E_u$ | – | 154 | IR | $x, y$ | 0.45 | 0.43 | 0.12 |
| $A_{2u}$ | – | 287 | IR | $z$ | 0.43 | 0.52 | 0.05 |
| $E_g$ | 520$^a$ | 485 | Raman | $xx - yy, xy, xz, yz$ | 0.00 | 0.00 | 1.00 |
| $E_u$ | 645 | 627 | IR | $x, y$ | 0.00 | 0.28 | 0.72 |
| $A_{1g}$ | 712$^a$ | 639 | Raman | $xx + yy, zz$ | 0.00 | 0.00 | 1.00 |
| $A_{2u}$ | 725$^a$ | 661 | IR | $z$ | 0.03 | 0.18 | 0.79 |

[a] Ref. 13.

While the calculated frequencies are in good agreement with a previous calculation [14], they may not reproduce the $A_{1g}$ and $A_{2u}$ modes observed above 700 cm$^{-1}$, which appear to be better described by pseudopotential techniques [15].

* homes@bnl.gov
† andy.mackenzie@cpfs.mpg.de
[1] Robert D. Shannon, Donald Burl Rogers, and Charles T. Prewitt, "Chemistry of noble metal oxides. I. Syntheses and properties of ABO2 delafossite compounds," Inorg. Chem. **10**, 713–718 (1971).
[2] D. J. Singh, *Planewaves, Pseudopotentials and the LAPW method* (Kluwer Adademic, Boston, 1994).
[3] David Singh, "Ground-state properties of lanthanum: Treatment of extended-core states," Phys. Rev. B **43**, 6388–6392 (1991).
[4] P. Blaha, K. Schwarz, G. K. H. Madsen, D. Kvasnicka and J. Luitz, WIEN2k, *An augmented plane wave plus local orbitals program for calculating crystal properties* (Techn. Universität Wien, Austria, 2001).

[5] R. Seshadri, C. Felser, K. Thieme, and W. Tremel, "Metal-Metal Bonding and Metallic Behavior in Some $ABO_2$ Delafossites," Chem. Mater. **10**, 2189–2196 (1998).
[6] Volker Eyert, Raymond Frésard, and Antoine Maignan, "On the Metallic Conductivity of the Delafossites $PdCoO_2$ and $PtCoO_2$," Chem. Mater. **20**, 2370–2373 (2008).
[7] Kyoo Kim, Hong Chul Choi, and B. I. Min, "Fermi surface and surface electronic structure of delafossite $PdCoO_2$," Phys. Rev. B **80**, 035116 (2009).
[8] Khuong P. Ong, Jia Zhang, John S. Tse, and Ping Wu, "Origin of anisotropy and metallic behavior in delafossite $PdCoO_2$," Phys. Rev. B **81**, 115120 (2010).
[9] Han-Jin Noh, Jinwon Jeong, Jinhwan Jeong, En-Jin Cho, Sung Baek Kim, Kyoo Kim, B. I. Min, and Hyeong-Do Kim, "Anisotropic Electric Conductivity of Delafossite $PdCoO_2$ Studied by Angle-Resolved Photoemission Spectroscopy," Phys. Rev. Lett. **102**, 256404 (2009).
[10] Clifford W. Hicks, Alexandra S. Gibbs, Andrew P. Mackenzie, Hiroshi Takatsu, Yoshiteru Maeno, and Edward A. Yelland, "Quantum Oscillations and High Carrier Mobility in the Delafossite $PdCoO_2$," Phys. Rev. Lett. **109**, 116401 (2012).
[11] Claudia Ambrosch-Draxl and Jorge O. Sofo, "Linear optical properties of solids within the full-potential linearized augmented planewave method," Comp. Phys. Commun. **175**, 1–14 (2006).
[12] K. Parlinksi, Software PHONON (2003).
[13] Hiroshi Takatsu, Shingo Yonezawa, Shinichiro Mouri, Satoru Nakatsuji, Koichiro Tanaka, and Yoshiteru Maeno, "Roles of High-Frequency Optical Phonons in the Physical Properties of the Conductive Delafossite $PdCoO_2$," J. Phys. Soc. Jpn. **76**, 104701 (2007).
[14] Long Cheng, Qing-Bo Yan, and Ming Hu, "The role of phonon-phonon and electron-phonon scattering in thermal transport in $PdCoO_2$," Phys. Chem. Chem. Phys. **19**, 21714–21721 (2017).
[15] S. Kumar, H.C. Gupta, and Karandeep, "First principles study of structural, bonding and vibrational properties of $PtCoO_2$, $PdCoO_2$ and $PdRhO_2$ metallic delafossites," J. Phys. Chem. Solids **74**, 305–310 (2013).
